# Supplementary material for: Fairness in Social Influence Maximization via Optimal Transport
Source: arXiv:2406.17736 source file (2025-01-30)
Supplement: Supplementary file 1 [file plot_comparison_metrics_appendix.pdf]

AH, TODO,  $|S| = 6$

Optimal transport fairness

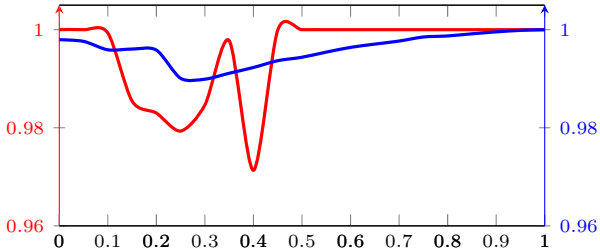

Conduction Probability

Equity (diff. in exp. outreach)

APS, bas\_d,  $|S| = 15$

Optimal transport fairness

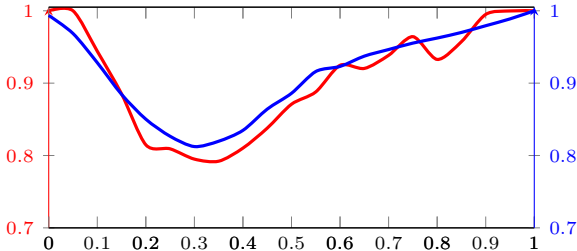

Equity (diff. in exp. outreach)

Conduction Probability

APS, bas\_g,  $|S| = 15$

Optimal transport fairness

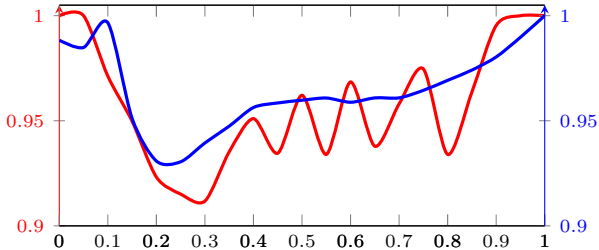

Equity (diff. in exp. outreach)

Conduction Probability

AV\_0, bas\_g,  $|S| = 20$

Optimal transport fairness

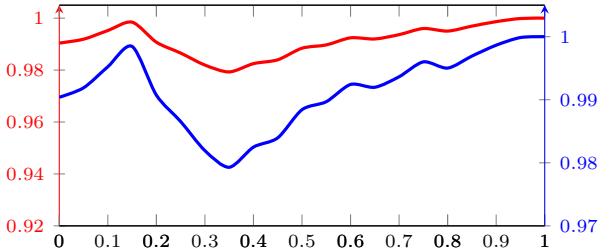

Conduction Probability

Equity (diff. in exp. outreach)

DZ, bas\_g,  $|S| = 50$

Optimal transport fairness

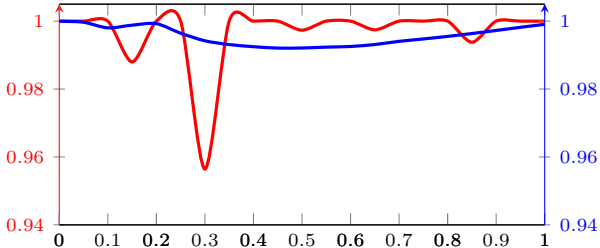

Equity (diff. in exp. outreach)

Conduction Probability

HS, bas\_g,  $|S| = 6$

Optimal transport fairness

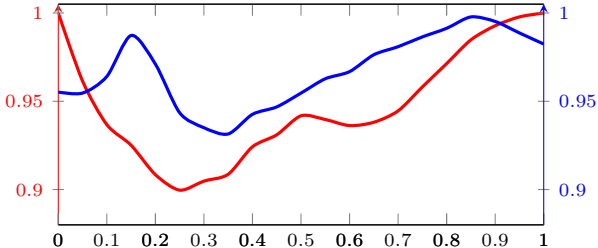

Conduction Probability

Equity (diff. in exp. outreach)

IV, bas\_g,  $|S| = 2$

Optimal transport fairness

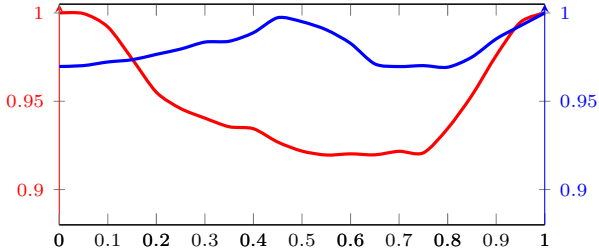

Equity (diff. in exp. outreach)

Conduction Probability
